# Supplementary material for: PIETRA: Physics-Informed Evidential Learning for Traversing Out-of-Distribution Terrain
Source: arXiv:2409.03005 source file (2024-12-24)
Supplement: Supplementary file 1 [file appendix.tex]

\section{Closed-Form $\uemdsq$ Loss~\cite{cai2024evora}}\label{appendix:uemdsq_details_and_entropy}

Given a Dirichlet distribution $q = \dir(\bm{\beta})$ and the target PMF $\mathbf{y}$, a closed-form expression exists for $L^{\uemdsq}(q, \mathbf{y})$:
\begin{align}
&L^{\uemdsq} \big(q, \mathbf{y}\big) \defeq \E_{\mathbf{p}\sim q} \big[ \emdsq (\mathbf{p}, \mathbf{y}) \big]\\
&= \cumsum(\overline{\mathbf{p}})\tr \frac{\cumsum(\bm{\beta})+\mathbf{1}_B}{\beta_0+1} + (\cumsum(\mathbf{y})- 2\ \cumsum(\overline{\mathbf{p}})\tr )\tr \cumsum(\mathbf{y})  \label{eq:uemd2}
\end{align}
where $\overline{\mathbf{p}}=\E_{\mathbf{p}\sim q}[\mathbf{p}]$.
